# Supplementary material for: Exact Electrostatic Theory of Fermi-Energy Response at Metallic Interfaces
Source: arXiv:2601.05660 ancillary file (2026-09-25)
Supplement: Supplementary file 1 [file suppl_mat.pdf]

# Exact Theory of Fermi-Energy Response at Metallic Interfaces – Supplemental Material

Théophane Bernhard and Andrea Grisafi*
*Physicochimie des Électrolytes et Nanosystèmes Interfaciaux, Sorbonne Université, CNRS, F-75005 Paris, France*

### Formal equivalence between finite-charge and finite-field approaches

We here provide a more thorough demonstration about the formal equivalence between finite-charge and finite-field approaches for the central finite-difference calculation of Fukui functions. We report them here for completeness:

$$f_{\Delta N}(\mathbf{r}) = \lim_{\Delta N \to 0} \frac{\Delta\rho_{+\Delta N}(\mathbf{r}) - \Delta\rho_{-\Delta N}(\mathbf{r})}{4\, Q_{\Delta N}} \tag{S1}$$

$$f_{\varepsilon_z}(\mathbf{r}) = \lim_{\varepsilon_z \to 0} \frac{\Delta\rho_{+\varepsilon_z}(\mathbf{r}) - \Delta\rho_{-\varepsilon_z}(\mathbf{r})}{4\, Q_{\varepsilon_z}}\,. \tag{S2}$$

While these equations generally apply for any given metallic interface, namely left and right hand side of the slab, a distinction must be made when comparing the two calculation pathways at the two sides. From the discussion reported in the main text, in particular, it is reasonable to perform a pairwise comparison between physically analogous terms in Eq. (S1) and Eq. (S2) associated with interfaces of equivalent number label and color indicated in Fig. 1. The argument is based on the idea that it is always possible to choose the value of $\varepsilon_z$ so that the pairs of highlighted interfaces are physically indistinguishable from each other. In fact, because of perfect electrostatic screening in the metal interior, each interface will feel the field of the complementary interfacial charge distribution as a uniform surface charge – as implied from conventional multipole expansions. For example, given a surface charge density $\sigma$, the right interface under an addition of electronic charge – blue area (2) in Fig. 1 – will be subject to an external field of $E_{\text{ext}} = 2\pi\sigma$, which corresponds to the net external field in the finite-field approach when choosing $\varepsilon_z = 4\pi\sigma$, i.e., $E_{\text{ext}} = \varepsilon_z - 2\pi\sigma = 2\pi\sigma$. Importantly, this equivalence is not restricted to the case of an isolated metallic slab, as the value of $\varepsilon_z$ can be adjusted to absorb any additional linear polarization term originated sufficiently far from the relevant interface region. This includes field-induced polarizations originated in the insulating region of the complementary side of the slab, as well as polarizations associated with the interaction along $z$ with the system's periodic images (in case 3D-periodicity is enforced). Since the electron density variation $\Delta\rho(\mathbf{r})$ at each interface is normalized by the corresponding amount of total surface charge $Q$, the actual finite-field value is indeed irrelevant. Therefore, we find that the two paths of Eq. (S1) and Eq. (S2) must lead to the same result for any sufficiently small value of $\Delta N$ and $\varepsilon_z$, respectively:

$$\begin{aligned}
f^{\mathrm{L}}_{\Delta N}(\mathbf{r}) &= \frac{1}{4}\left[\underbrace{+\frac{\Delta\rho^{\mathrm{L}}_{\Delta N}(\mathbf{r})}{|Q_{\Delta N}|}}_{(1)} \underbrace{-\frac{\Delta\rho^{\mathrm{L}}_{-\Delta N}(\mathbf{r})}{|Q_{\Delta N}|}}_{(3)}\right], \qquad
f^{\mathrm{R}}_{\Delta N}(\mathbf{r}) = \frac{1}{4}\left[\underbrace{+\frac{\Delta\rho^{\mathrm{R}}_{\Delta N}(\mathbf{r})}{|Q_{\Delta N}|}}_{(2)} \underbrace{-\frac{\Delta\rho^{\mathrm{R}}_{-\Delta N}(\mathbf{r})}{|Q_{\Delta N}|}}_{(4)}\right], \\
f^{\mathrm{L}}_{\varepsilon_z}(\mathbf{r}) &= \frac{1}{4}\left[\underbrace{-\frac{\Delta\rho^{\mathrm{L}}_{+\varepsilon_z}(\mathbf{r})}{|Q_{\varepsilon_z}|}}_{(3)} \underbrace{+\frac{\Delta\rho^{\mathrm{L}}_{-\varepsilon_z}(\mathbf{r})}{|Q_{\varepsilon_z}|}}_{(1)}\right], \qquad
f^{\mathrm{R}}_{\varepsilon_z}(\mathbf{r}) = \frac{1}{4}\left[\underbrace{+\frac{\Delta\rho^{\mathrm{R}}_{+\varepsilon_z}(\mathbf{r})}{|Q_{\varepsilon_z}|}}_{(2)} \underbrace{-\frac{\Delta\rho^{\mathrm{R}}_{-\varepsilon_z}(\mathbf{r})}{|Q_{\varepsilon_z}|}}_{(4)}\right].
\end{aligned} \tag{S3}$$

## Connection with dielectric response function

We here draw the connection between our result and the conventional dielectric response picture provided by the static electronic susceptibility $\chi(\mathbf{r}, \mathbf{r}')$. In this context, the response of the self-consistent electrostatic potential $v(\mathbf{r})$ to the external potential $v_{\text{ext}}(\mathbf{r})$ can be expressed from the inverse of the dielectric function $\epsilon(\mathbf{r}, \mathbf{r}')$:

$$\Delta v(\mathbf{r}) = \int \mathrm{d}\mathbf{r}' \, \epsilon^{-1}(\mathbf{r}, \mathbf{r}') \, \Delta v_{\text{ext}}(\mathbf{r}') \, , \tag{S4}$$

where we used the known definition for $\epsilon^{-1} = 1 + v_C \star \chi$, with $v_C$ the Coulomb potential [1]. Because of perfect screening, $\Delta v(\mathbf{r})$ in the interior of the electronic conductor must correspond to a rigid shift $\Delta V_{\text{bulk}}$ equal to the Fermi-level variation, i.e., $\Delta E_{\text{F}} \simeq \Delta V_{\text{bulk}} = \Delta v(\mathbf{r}_{\text{bulk}})$, with $\mathbf{r}_{\text{bulk}}$ indicating any point in the metallic bulk. We finally obtain a direct relationship between $\epsilon^{-1}$ and the Fukui function:

$$f(\mathbf{r}) = \frac{\delta E_{\text{F}}}{\delta v_{\text{ext}}(\mathbf{r})} \simeq \frac{\delta v(\mathbf{r}_{\text{bulk}})}{\delta v_{\text{ext}}(\mathbf{r})} = \epsilon^{-1}(\mathbf{r}_{\text{bulk}}, \mathbf{r}) \, . \tag{S5}$$

## Computational details for Pt-surfaces calculation of Fukui functions

All three platinum surfaces considered in this work are built starting from a $4 \times 4 \times 7$ Pt(111) slab. A full geometry relaxation is performed at the DFT/PBE level [2] with a double-$\zeta$ (DZVP) basis set [3] and GTH pseudopotentials [4], using the CP2K electronic-structure program. [5] The finite-field calculation of Fukui functions was performed following Eq. (S2), by applying positive and negative electric fields along $z$ of $\varepsilon_z = \pm 0.01$ V/Å. For this, a triple-$\zeta$ (TZVP) basis set with a $3 \times 3 \times 1$ $k$-points grid was adopted to better represent the response of the electron density. Moreover, the Martyna-Tuckerman scheme was adopted to screen the dipolar field of the system's periodic images along the nonconductive direction $z$ [6]. The central finite-difference calculation between electron densities was performed directly on the real-space grid used for the DFT calculation. The amount of charge $Q$ accumulated at the surface, required for the functions normalization, was then consistently computed by integrating the electron density variation $\Delta\rho$ from the metallic bulk to the vacuum region as in Eq. (S2).

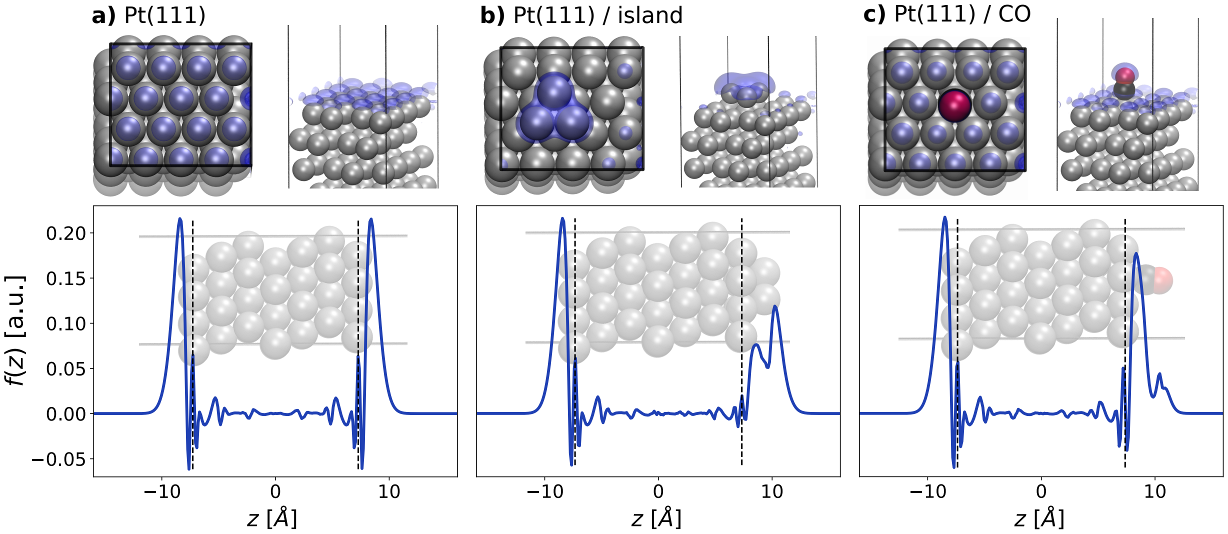


FIG. S1. Computed Fukui functions for three relaxed Pt(111) surfaces, reported as a spatial integral over the periodic $xy$ plane: a) bare metal slab, b) metal slab with a 3 Pt-atoms island, c) metal slab with an adsorbed CO molecule on a top Pt-site. Vertical dashed lines indicate the positions of the surface platinum layers, as also depicted by the structures background images. Identical profiles on the left hand side of the slabs expose the nature of Fukui functions as local surface properties.

In Fig. S1, the computed Fukui functions of the three types of platinum surfaces are reported along $z$ by integrating $f(\boldsymbol{r})$ over the periodic $xy$ plane. We notice that the Fukui function profiles mirror the response of the electron density under the applied field – displaying the typical electronic spillover peaks right beyond the outermost metal layers. When compared with the bare Pt(111) case, the defective slab geometry displays a pronounced response

at the location of the Pt-island (Fig. S1-b), while the CO adsorption appears to slightly smear the response of the main metal peak towards the oxygen atom (Fig. S1-c). Notably, the Fukui function profiles on the left hand side of the slab (clean surface) are identical in the three cases, providing numerical evidence to the assumed independent nature of the response at each interface. The result obtained for the bare metal slab (Fig. S1-a) can be directly compared with what reported in Ref. [7], where different types of Fukui function calculations are performed using both corrected finite-charge approaches and LDOS approximations. We find that our result appears in qualitative agreement with the right-derivative Fukui function computed with the finite-charge approach corrected with an exact coulomb cutoff (ECC) scheme [8, 9], while all other methods yield some qualitative differences that are primarily related to a nonvanishing behaviour in the metallic bulk. We further notice a loose qualitative agreement of our Fukui functions with those reported in Ref. [10], where both the bare Pt(111) slab and the CO adsorption case were studied using a suitable electrochemical correction scheme to the finite-charge approach.

## Computational details for the Ag/water calculation of Fukui functions

The Ag/water interface considered in this work consisted in a $4 \times 4 \times 7$ Ag(111) slab in contact with 256 water molecules under 3D periodic boundary conditions. The box size along $z$ is set as $L_z = 83.0$ Å, thereby comprising liquid water layers that totally fill the simulation box, and that extend for approximately 34 Å on each side of the metallic slab. The configurational space at room temperature is sampled via a classical molecular dynamics (MD) simulation using the MetalWalls program [11]. The simulation is run for 200 ps in timesteps of 2 fs using a Nosé-Hoover thermostat [12]. Classical interactions are represented with a SPC/E water model [13], and using the silver Lennard-Jones parameters reported in Ref. [14]. Classical charges on the Ag atoms are represented using a Gaussian width of $\eta_{\mathrm{Ag}} = 1.1$ Å, following the Siepmann-Sprik model [15]. The finite-field calculation of Fukui functions is performed on a total of 400 independent frames selected every 0.5 ps from the classical trajectory. To limit the computational burden, we perform the DFT calculations at the Γ-point using the PBE functional and a double-$\zeta$ basis set. This level of theory has proven to be enough to yield a potential of zero charge (PZC) at the Ag(111)/water interface that is in good agreement with experiments [16].

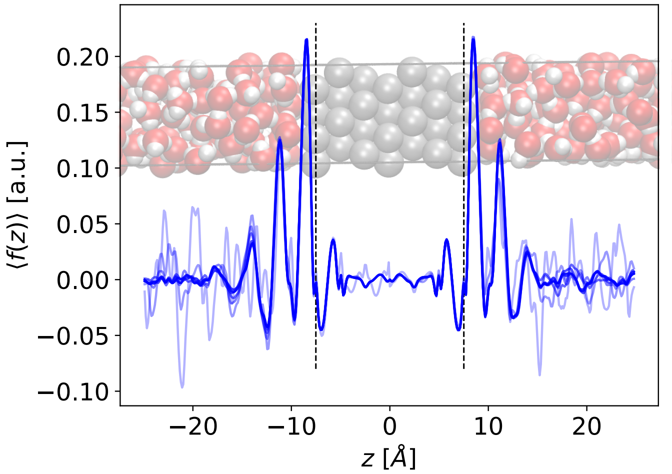


FIG. S2. Computed Fukui functions at a Ag(111)/water interface, reported as a statistical average over a classical molecular dynamics simulation. Curves of higher opacity correspond to ensemble averages performed over increasingly longer trajectories, up to a maximum of 200 ps. Vertical dashed lines indicate the positions of the surface silver atoms, consistently with the location of the system's background image.

The integrated Fukui functions, $f(z)$, are reported in Fig. S2 as a statistical average over increasingly longer trajectories. In contrast with the case of isolated surfaces, the instantaneous profiles display a nonvanishing behaviour in the electronically insulating region, which is ultimately due to the electrostatic polarization of water molecules. An analogous effect is also to be expected as a consequence of the metal charging whenever computing Fukui functions with conventional approaches; an example of this is reported in Ref. [10]. Upon performing the ensemble average over the simulated trajectory, we find a smooth oscillatory profile that decays into the water bulk region, exposing the interfacial nature of the Fermi-energy response at thermal equilibrium.

**Modified Poisson-Boltzmann model for the Ag(111)/NaF(aq) interface**

We report here a detailed description of the modified Poisson-Boltzmann model [17] used in this work. We start by representing the electrode charge density, $\rho_Q^{\mathrm{M}}(z)$, via a fixed Gaussian distribution centered on the surface metal layers, such that, $\int dz\, \rho_Q^{\mathrm{M}}(z) = \sigma_{\mathrm{M}}$ is the surface charge density of the electrode, set as an input parameter of the model. The Gaussian width $\eta_{\mathrm{Ag}}$ is chosen as equivalent to that already adopted in the previous section. We then express the ionic charge density distribution, $\rho_Q^{\mathrm{ions}}(z)$, using the Kornyshev correction to the Poisson-Boltzmann equations, suitable to account for the saturation of ionic density at the interface [17]. In particular, we define the equilibrium charge density distribution of the electrolyte at the electrode surface as follows:

$$\rho_Q^{\mathrm{ions}}(z) = \bar{\rho}\left[e^{-\beta\left(V_{\mathrm{LJ}}^{+}(z)+\phi(z)\right)} - e^{-\beta\left(V_{\mathrm{LJ}}^{-}(z)-\phi(z)\right)}\right] \times \left\{1+\frac{\gamma}{2}\left[e^{-\frac{\beta}{2}\left(V_{\mathrm{LJ}}^{+}(z)+\phi(z)\right)} - e^{-\frac{\beta}{2}\left(V_{\mathrm{LJ}}^{-}(z)-\phi(z)\right)}\right]^2\right\}^{-1}, \tag{S6}$$

where we used the symbol $\phi(z)$ to indicate the thermally-averaged electrostatic potential (indicated by $\langle\Delta\phi(z)\rangle$ in the main text) for brevity. $\beta$ is the inverse of room temperature, $\bar{\rho}$ is the bulk ionic density, and $V_{\mathrm{LJ}}^{\pm}(z)$ is the 9-3 Lennard-Jones pair-potential between ions and the Ag(111) surface atoms. Finally, $\gamma$ controls the degree of ionic saturation and it is defined from the ratio of the bulk ionic density and the average close-packing density, $\bar{\rho}_{\mathrm{max}}$, i.e., $\gamma = 2\,\bar{\rho}/\bar{\rho}_{\mathrm{max}}$. In practice, this is often used as an adjustable parameter of the model. Here, we consider a close-packing density of $\bar{\rho}_{\mathrm{max}} = 0.013$ ions/Å$^3$, corresponding to an order-of-magnitude estimate based on an effective hydration radius of $Na^+$ and $F^-$ ions adsorbed at the Ag(111) surface of $r_{\mathrm{eff}} \sim 2.4$ Å.

The 9-3 Lennard-Jones potential is defined from the planar integral along the $xy$-plane of the 12-6 Lennard-Jones pair-potential between the ions (±) and the Ag(111) surface atoms:

$$V_{\mathrm{LJ}}^{\pm}(z) = \frac{2\pi}{3}\bar{\rho}_s\sigma_{\pm}^3\epsilon_{\pm}\left[\frac{2}{15}\left(\frac{\sigma_{\pm}}{z-z_0}\right)^9 - \left(\frac{\sigma_{\pm}}{z-z_0}\right)^3\right] \tag{S7}$$

where $\bar{\rho}_s = 0.059$ atoms/Å$^3$ is the average number density of silver atoms, $z_0$ is the position of the surface metal layer, while $\epsilon_{\pm}$ and $\sigma_{\pm}$ are the Lennard-Jones parameters, tuned to account for physical potential depths and minimum adsorption distances. The potential depth is derived from the 12-6 Lennard-Jones parameters of $Na^+$ and $F^-$ fitted for a SPC/E water model [18], combined with the 12-6 Lennard-Jones parameters of the Ag(111) slab [14]. The minimum adsorption distance of $Na^+$ and $F^-$ from the Ag(111) surface is estimated from the *ab initio* molecular dynamics (AIMD) ionic distributions reported in Ref. [19]. The resulting 9-3 Lennard-Jones profiles are shown in Fig. S3. We note that the location of the $Na^+$ minimum at a farther distance than that of $F^-$ effectively takes into account the water solvation structure included in the AIMD simulation, which is not explicitly treated here.

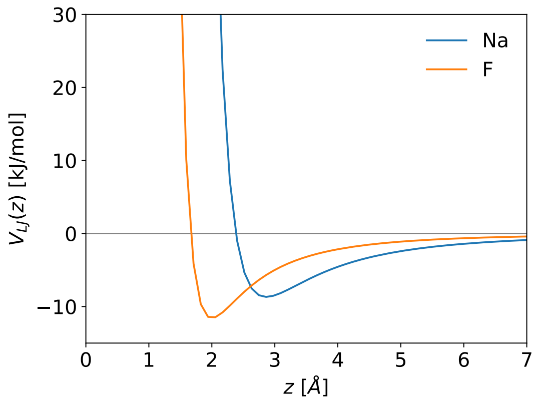


FIG. S3. 9-3 Lennard-Jones profile describing the short-range interaction between $Na^+$ and $F^-$, and the Ag(111) surface.

From the previous definitions, the electrostatic potential profile is found by solving the generalized Poisson equation with an inhomogeneous dielectric:

$$\frac{d}{dz}\left[\epsilon_r^{\mathrm{w}}(z)\,\phi'(z)\right] = -4\pi\left[\rho_Q^{\mathrm{M}}(z) + \rho_Q^{\mathrm{ions}}(z)\right], \tag{S8}$$

with $\epsilon_r^{\mathrm{w}}(z)$ the relative dielectric function of water at the interface. The latter is defined as a smooth sigmoid function that goes from $\epsilon_r^{\mathrm{w}} = 6$ in the proximity of the electrode surface [20, 21] to $\epsilon_r^{\mathrm{w}} = 78$ after a distance of $\sim 1.2$ nm that comprises the first three solvation layers. In practice, we set $z = 0$ in the metallic bulk and $z \to \infty$ in the asymptotic liquid bulk regime. Finally, solving Eq. (S8) under the boundary conditions $\phi'(0) = \phi'(\infty) = 0$ is enough to guarantee that the ionic charge distribution perfectly screens the electrode surface charge, i.e., $\int dz\, \rho_Q^{\mathrm{ions}}(z) = -\sigma_{\mathrm{M}}$, making the interface overall electroneutral.

The resulting electrostatic potential profiles are reported in Fig. S4-b for an example NaF concentration of $\bar{\rho} = 0.1$ M. For both positive and negative values of $\sigma_{\mathrm{M}}$, we observe the characteristic dipolar jump of $\Delta\phi(z)$ associated with the formation of the electrical double layer. In Fig. S4-a, we also report the thermal average of the Fukui function profile of the Ag(111)/water interface adopted as reference PZC state. For that, we perform the sum of $\langle f(z) \rangle$ computed at the two equivalent interfaces depicted in Fig. S2, allowing us to double the amount of statistics while preserving the unitary normalization required for the Fermi-energy response. This is made possible by the inherent nature of Fukui functions as single-interface properties, as derived from our theory. From a direct comparison with $\Delta\phi(z)$, we note how the largest local variations of electrostatic potential fall in correspondence of the main Fukui function peak, remarking the critical importance of disposing of an accurate calculation of $f(z)$ at the interface.

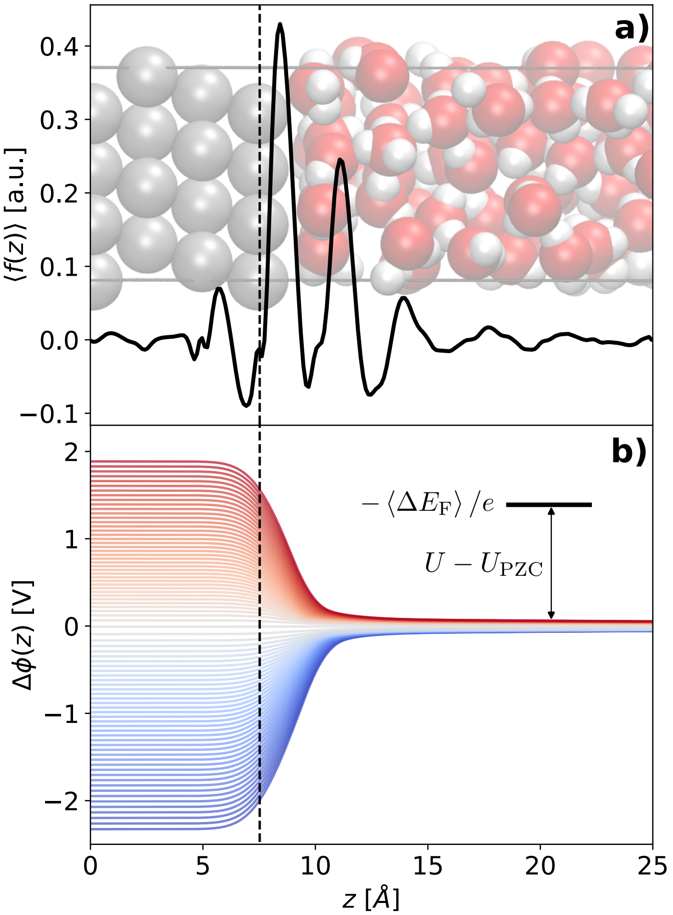


FIG. S4. Top panel (a): Thermally averaged Fukui function integrated over the $xy$-plane of the Ag(111)/water interface at zero surface charge (background image) used as linear-response function for the system's Fermi energy. Bottom panel (b): Classical EDL potential formed at the interface between an aqueous solution of NaF 0.1M and the Ag(111) electrode at varying surface charges. A color gradient from blue to red is used to indicate negative and positive potential profiles, respectively. Inset: schematic representation of the electrode potential calculation. Dashed line: $z$-position of the Ag surface atoms by setting the central layer of the metal slab at $z = 0$.

* andrea.grisafi@sorbonne-universite.fr

[S1] R. Martin, L. Reining, and D. Ceperley, *Interacting Electrons: Theory and Computational Approaches* (Cambridge University Press, 2016).

[S2] J. P. Perdew, K. Burke, and M. Ernzerhof, Generalized Gradient Approximation made simple, Phys. Rev. Lett. **77**, 3865 (1996).

[S3] J. VandeVondele and J. Hutter, Gaussian basis sets for accurate calculations on molecular systems in gas and condensed phases, The Journal of Chemical Physics **127**, 114105 (2007).

[S4] S. Goedecker, M. Teter, and J. Hutter, Separable dual-space gaussian pseudopotentials, Phys. Rev. B **54**, 1703 (1996).

[S5] T. D. Kühne, M. Iannuzzi, M. Del Ben, V. V. Rybkin, P. Seewald, F. Stein, T. Laino, R. Z. Khaliullin, O. Schütt, F. Schiffmann, D. Golze, J. Wilhelm, S. Chulkov, M. H. Bani-Hashemian, V. Weber, U. Borštnik, M. Taillefumier, A. S. Jakobovits, A. Lazzaro, H. Pabst, T. Müller, R. Schade, M. Guidon, S. Andermatt, N. Holmberg, G. K. Schenter, A. Hehn, A. Bussy, F. Belleflamme, G. Tabacchi, A. Glöß, M. Lass, I. Bethune, C. J. Mundy, C. Plessl, M. Watkins, J. VandeVondele, M. Krack, and J. Hutter, Cp2k: An electronic structure and molecular dynamics software package - quickstep: Efficient and accurate electronic structure calculations, The Journal of Chemical Physics **152**, 194103 (2020).

[S6] P. Mináry, M. E. Tuckerman, K. A. Pihakari, and G. J. Martyna, A new reciprocal space based treatment of long range interactions on surfaces, The Journal of Chemical Physics **116**, 5351 (2002).

[S7] N. F. Barrera, J. Cabezas-Escares, F. Muñoz, W. A. Muriel, T. Gómez, M. Calatayud, and C. Cárdenas, Fukui function and fukui potential for solid-state chemistry: Application to surface reactivity, Journal of Chemical Theory and Computation **21**, 3187 (2025).

[S8] C. A. Rozzi, D. Varsano, A. Marini, E. K. U. Gross, and A. Rubio, Exact coulomb cutoff technique for supercell calculations, Phys. Rev. B **73**, 205119 (2006).

[S9] M. R. Jarvis, I. D. White, R. W. Godby, and M. C. Payne, Supercell technique for total-energy calculations of finite charged and polar systems, Phys. Rev. B **56**, 14972 (1997).

[S10] J.-S. Filhol and M.-L. Doublet, Conceptual surface electrochemistry and new redox descriptors, The Journal of Physical Chemistry C **118**, 19023 (2014).

[S11] A. Coretti, C. Bacon, R. Berthin, A. Serva, L. Scalfi, I. Chubak, K. Goloviznina, M. Haefele, A. Marin-Laflèche, B. Rotenberg, S. Bonella, and M. Salanne, MetalWalls: simulating electrochemical interfaces between polarizable electrolytes and metallic electrodes, J. Chem. Phys. **157**, 184801 (2022).

[S12] S. Nosé, A unified formulation of the constant temperature molecular dynamics methods, J. Chem. Phys. **81**, 511 (1984).

[S13] H. J. C. Berendsen, J. R. Grigera, and T. P. Straatsma, The missing term in effective pair potentials, The Journal of Physical Chemistry **91**, 6269 (1987).

[S14] H. Heinz, R. A. Vaia, B. L. Farmer, and R. R. Naik, Accurate simulation of surfaces and interfaces of face-centered cubic metals using 126 and 96 lennard-jones potentials, The Journal of Physical Chemistry C **112**, 17281 (2008).

[S15] J. I. Siepmann and M. Sprik, Influence of surface topology and electrostatic potential on water/electrode systems, The Journal of Chemical Physics **102**, 511 (1995).

[S16] J. Le, M. Iannuzzi, A. Cuesta, and J. Cheng, Determining potentials of zero charge of metal electrodes versus the standard hydrogen electrode from density-functional-theory-based molecular dynamics, Phys. Rev. Lett. **119**, 016801 (2017).

[S17] A. A. Kornyshev, Double-layer in ionic liquids: Paradigm change?, The Journal of Physical Chemistry B **111**, 5545 (2007).

[S18] S. H. Lee and J. C. Rasaiah, Molecular dynamics simulation of ion mobility. 2. alkali metal and halide ions using the spc/e model for water at 25 °c, The Journal of Physical Chemistry **100**, 1420 (1996).

[S19] L. Li, Y.-P. Liu, J.-B. Le, and J. Cheng, Unraveling molecular structures and ion effects of electric double layers at metal water interfaces, Cell Reports Physical Science **3**, 100759 (2022).

[S20] J. Fiedler, M. Boström, C. Persson, I. Brevik, R. Corkery, S. Y. Buhmann, and D. F. Parsons, Full-spectrum high-resolution modeling of the dielectric function of water, The Journal of Physical Chemistry B **124**, 3103 (2020).

[S21] J.-X. Zhu, J. Cheng, and K. Doblhoff-Dier, Dielectric profile at the pt(111)/water interface, The Journal of Chemical Physics **162**, 024702 (2025).
